# Supplementary material for: MoSSP: A Momentum-Based Single-Loop Stochastic Penalty Method for Nonconvex Constrained DC-Regularized Optimization
Source: arXiv:2605.29635 source file (2026-05-28)
Supplement: Supplementary file 1 [file DME_solutions_related.tex]

\section{Appendix: Solution Correspondence for Difference-of-Moreau-Envelopes}
\label{appendix: DME properties}
In this section, we provide the complete theoretical relationship between solutions of Problem~\eqref{wcu} and its DME surrogate $\min\limits_{\bz \in \RR^n} F_\mu(\bz)$ with rigorous proofs. We first present essential mathematical tools.

\subsection{Infimal Convolution and Toland Duality}

\paragraph{\textbf{Infimal convolution \cite{moreau1971weak}.}} Let $f,\theta : \RR^n \to (-\infty,+\infty]$ be proper lower semicontinuous functions.
For any \(\bz \in \RR^n\), the infimal convolution is defined by
\begin{align}
% \label{Eq: definition infimal convolution}
(f \square \theta)(\bz) := \inf_{\bx \in \RR^n} \left\{f(\bx) + \theta(\bx - \bz)\right\}. \notag
\end{align}
When $\theta(\cdot) = \frac{1}{2\mu}\|\cdot\|^2$ for some $\mu>0$, this reduces to the \textit{Moreau envelope}:
\begin{align}
% \label{Eq: Moreau as infimal convolution}
\mathcal{M}_{\mu \phi}(\bz) = \left(\phi \square \frac{1}{2\mu}\|\cdot\|^2\right)(\bz). \notag
\end{align}
A key property \cite{borwein2006convex} states that conjugation transforms infimal convolution into summation:
\begin{align}
(f_1 \square f_2)^* = f_1^* + f_2^*, \notag
\end{align}
where, for any $\by \in \RR^n$,
\begin{align}
  f^*(\by) := \sup_{\bx \in \RR^n} \{\langle \by, \bx\rangle - f(\bx)\} \notag
\end{align}
denotes the Fenchel conjugate function of $f$.
This yields the conjugate function of the \textit{Moreau envelope}:
\begin{align}
% \label{Eq: conjugate Moreau envelope}
\mathcal{M}_{\mu \phi}^*(\by) = \phi^*(\by) + \frac{1}{2\mu}\|\by\|^2, \quad \forall\,\by \in \RR^n.\notag
\end{align}

\paragraph{\textbf{Toland duality \cite{toland1978duality}.}} The Toland dual of the objective function of Problem~\eqref{wcu} is defined as
\begin{align}
\label{Eq: Toland dual function}
F^\circ(\by) = g^*(\by) - \phi^*(\by). 
\end{align}
A key duality property of \(F\) and \(F_{\mu}\) is
\begin{align}
\label{Eq: Toland duality equality}
\inf_{\bx } F(\bx) = \inf_{\by} F^\circ(\by).
\end{align}

\subsection{Solution Correspondence Theory}
\label{App: Solution Correspondence Theory}
We now extend the solution correspondence theory of \citet{hiriart1991regularize} to the \textbf{weakly convex} setting. Let us define the optimal values $\hat{F} = \min\limits_{\bx} F(\bx)$ and $\hat{F}_{\mu} = \min\limits_{\bz} F_{\mu}(\bz)$, with the corresponding minimizer sets $\mathcal{X}_{F} = \argmin\limits_{\bx} F(\bx)$ and $\mathcal{X}_{F_{\mu}} = \argmin\limits_{\bz} F_{\mu}(\bz)$. A crucial characterization concerns the preimage of the proximal operator.
\paragraph{\textbf{Preimage characterization.}}
Let $f : \RR^n \to (-\infty,+\infty]$ be a proper lower semicontinuous function.
For any $\bx \in \RR^n$ with $\partial f(\bx) \neq \emptyset$ and any $\bxi \in \partial f(\bx)$, it holds that, for any $\mu > 0$,
\begin{align}
\label{Eq: the preimage of moreau envelope}
\mathrm{prox}_{\mu f}(\bx + \mu \bxi) = \bx.
\end{align}
This follows directly from the optimality condition of the Moreau envelope or, equivalently, from \eqref{Eq: the gradient of Moreau envelope}.

\begin{proposition}[Stationary Point and Global Minimizer Correspondence]
\label{Prop: correspondence of stationary point and global minimizer}
Consider problem \eqref{wcu}. For any $0 < \mu < \frac{1}{m_{\phi}}$, the following holds:

\textbf{(i) Stationary point correspondence.} If $\nabla F_{\mu}(\bar{\bz}) = \mathbf{0}$, then $\bar{\bx} := \textrm{prox}_{\mu\phi}(\bar{\bz})$ is a critical point of $F$ with
\begin{align}
\label{Eq: stationary identity}
\textrm{prox}_{\mu\phi}(\bar{\bz}) = \textrm{prox}_{\mu g}(\bar{\bz}), \quad F(\bar{\bx}) = F_{\mu}(\bar{\bz}).
\end{align}
Conversely, if $\bar{\bx}$ is a critical point of $F$ and $\bar{\bxi} \in \partial\phi(\bar{\bx}) \cap \partial g(\bar{\bx})$, then $\bar{\bz} = \bar{\bx} + \mu \bar{\bxi}$ is a stationary point of $F_{\mu}$ with $\textrm{prox}_{\mu \phi}(\bar{\bz}) = \textrm{prox}_{\mu g}(\bar{\bz}) = \bar{\bx}$ and $F(\bar{\bx}) = F_{\mu}(\bar{\bz})$.

\textbf{(ii) Global minimizer correspondence.}
$\mathcal{X}_{F_{\mu}} \neq \emptyset$ and $\hat{F} = \hat{F}_{\mu}$. Furthermore, if $\bar{\bz} \in \mathcal{X}_{F_{\mu}}$, then $\textrm{prox}_{\mu \phi}(\bar{\bz}) \in \mathcal{X}_{F}$; conversely, if $\bar{\bx} \in \mathcal{X}_F$ and $\bar{\bxi} \in \partial\phi(\bar{\bx}) \cap \partial g(\bar{\bx})$, then $\bar{\bz} = \bar{\bx} + \mu \bar{\bxi} \in \mathcal{X}_{F_{\mu}}$.
\end{proposition}

\begin{proof}
\textbf{Proof of Claim \textbf{(i)}.} If $\nabla F_{\mu}(\bar{\bz}) = 0$, then it holds that
\begin{align}
\mu\nabla F_{\mu}(\bar{\bz}) = \textrm{prox}_{\mu g}(\bar{\bz}) - \textrm{prox}_{\mu\phi}(\bar{\bz}) = 0, \notag
\end{align}
establishing the first equality in \eqref{Eq: stationary identity}. The function value equality in \eqref{Eq: stationary identity} follows from
\begin{align}
F(\textrm{prox}_{\mu\phi}(\bar{\bz})) 
&= \phi(\textrm{prox}_{\mu\phi}(\bar{\bz})) 
   - g(\textrm{prox}_{\mu g}(\bar{\bz})) \notag \\
&= \left[\phi(\textrm{prox}_{\mu\phi}(\bar{\bz})) 
   + \frac{1}{2\mu}\|\bar{\bz} - \textrm{prox}_{\mu\phi}(\bar{\bz})\|^2 \right]  - \left[g(\textrm{prox}_{\mu g}(\bar{\bz})) 
   + \frac{1}{2\mu}\|\bar{\bz} - \textrm{prox}_{\mu g}(\bar{\bz})\|^2 \right] \notag \\
&= \mathcal{M}_{\mu\phi}(\bar{\bz}) - \mathcal{M}_{\mu g}(\bar{\bz})
   = F_\mu(\bar{\bz}). \notag
\end{align}

For the converse, let $\bar{\bx}$ be a critical point with $\bar{\bxi} \in \partial\phi(\bar{\bx}) \cap \partial g(\bar{\bx})$ and take $\bar{\bz} = \bar{\bx} + \mu \bar{\bxi}$. By \eqref{Eq: the preimage of moreau envelope}, one has $\textrm{prox}_{\mu \phi}(\bar{\bz}) = \textrm{prox}_{\mu g}(\bar{\bz}) = \bar{\bx}$, yielding $\nabla F_{\mu}(\bar{\bz}) = 0$. The value equality follows similarly.

\textbf{Proof of Claim \textbf{(ii)}.} Since $F_{\mu}$ is $L_{F_{\mu}}$-smooth and bounded below from \Cref{Prop: smoothness of DME} (iii), it is coercive, ensuring $\mathcal{X}_{F_{\mu}} \neq \emptyset$. 
% Recalling \eqref{Eq: Toland dual function}, the Toland's dual of $F_{\mu}$ is:
% \begin{align}
% F^{\circ}_{\mu}(\bz)&= \mathcal{M}_{\mu g}(\bz) - \mathcal{M}_{\mu \phi}(\bz) \notag \\
% &= \left(g^* + \frac{1}{2\mu}\|\cdot\|^2\right) - \left(\phi^* + \frac{1}{2\mu}\|\cdot\|^2\right) \notag \\
% &= g^* - \phi^* = F^{\circ}, \notag
% \end{align}
Recalling \eqref{Eq: Toland dual function}, the Toland dual of $F_{\mu}$ is
\begin{align}
F^{\circ}_{\mu}(\by)
  &= \mathcal{M}_{\mu g}^*(\by) - \mathcal{M}_{\mu \phi}^*(\by) \notag \\
  &= \bigl(g^* + \tfrac{1}{2\mu}\|\cdot\|^2\bigr)(\by)
     - \bigl(\phi^* + \tfrac{1}{2\mu}\|\cdot\|^2\bigr)(\by) \notag \\
  &= g^*(\by) - \phi^*(\by) = F^{\circ}(\by). \notag
\end{align}
Together with \eqref{Eq: Toland duality equality}, this yields the global minimum equivalence.
% \begin{align}
% % \label{Eq: optimal value equality}
% \hat{F}_{\mu} = \inf F_{\mu} = \inf F_{\mu}^\circ = \inf F^\circ = \inf F = \hat{F}. \notag
% \end{align}

For the minimizer correspondence, it is evident that if $\bar{\bz} \in \mathcal{X}_{F_{\mu}}$, then $\bar{\bz}$ is a stationary point. From \textbf{Claim {(i)}}, $\bar{\bx} := \textrm{prox}_{\mu \phi}(\bar{\bz})$ is a critical point with
\[
F(\bar{\bx}) = F_{\mu}(\bar{\bz}) = \hat{F}_{\mu} = \hat{F},
\] yielding $\bar{\bx} \in \mathcal{X}_F$. The converse follows similarly from the second part of \textbf{Claim} \textbf{(i)}.
\end{proof}

% \begin{remark}[Key implications]
% This proposition establishes that:
% \begin{enumerate}
% \item The mapping $\textrm{prox}_{\mu\phi}$ provides a bijection between stationary points of $F_{\mu}$ and critical points of $F$;
% \item Optimal values are preserved: $\hat{F}_{\mu} = \hat{F}$;
% \item The minimizer sets correspond bijectively via $\textrm{prox}_{\mu\phi}$.
% \end{enumerate}
% These properties are fundamental for developing algorithms that solve the smooth problem $\min F_{\mu}$ to find critical points of the nonsmooth problem $\min F$.
% \end{remark}

Moreover, while \citet{sun2023algorithms} established that a local minimizer of $F$ can be obtained from a local minimizer of $F_{\mu}$ under the condition that $g$ is smooth or has bounded subgradients, the following proposition completes this result by rigorously establishing a full equivalence relationship between their local minimizers.

\begin{proposition}[Local Minimizers Correspondence]
\label{Prop: correspondence of local minimizer}
Under the conditions in \Cref{Prop: correspondence of stationary point and global minimizer}, suppose either of the following conditions on $\partial g$ holds:

\textbf{(i).} $g$ is $L_g$-smooth,

\textbf{(ii).} $\sup\limits_{\xi_g \in \partial g} \|\xi_g\| \leq M_{\partial g}$ for some \(M_{\partial g} > 0\).

Then, $\bar{\bx} := \textrm{prox}_{\mu \phi}(\bar{\bz})$ is a local minimizer of $F$ with radius $r_{\bx}> 0$ if and only if for any $\bar{\bxi} \in \partial \phi(\bar{\bx}) \cap \partial g(\bar{\bx})$, $\bar{\bz} = \bar{\bx} + \mu \bar{\bxi}$ is a local minimizer of $F_{\mu}$ with radius $r_{\bz}> 0$, where $r_{\bx}$ and $r_{\bz}$ satisfy
\begin{align}
     \label{Eq: the relationship of rx and rz}
r_x =
\begin{cases}
  \dfrac{r_z}{\mu L_g + 1}, 
    & \text{if $g$ is $L_g$-smooth,} \\[0.3ex]
  \bigl(r_z - 2\mu M_{\partial g}\bigr)\vphantom{\dfrac{r_z}{\mu L_g + 1}}, 
    & \text{if $\sup_{\xi_g \in \partial g}\|\xi_g\|\le M_{\partial g}$ and $r_z > 2\mu M_{\partial g}$.}
\end{cases}
    \end{align}
\end{proposition}

\begin{proof}
We begin with the local minimizer property of \(\bar{\bx}\). If $\bar{\bx}$ is a local minimizer of $F$ with radius \(r_{\bx}\), for any $\bar{\bxi} \in \partial \phi(\bar{\bx}) \cap \partial g(\bar{\bx})$, let us define $\bar{\bz} = \bar{\bx} + \mu \bar{\bxi}$. By \Cref{Prop: correspondence of stationary point and global minimizer}, we have $\textrm{prox}_{\mu \phi}(\bar{\bz}) = \textrm{prox}_{\mu g}(\bar{\bz}) = \bar{\bx}$.
% For any $\bx$ with $\|\bx - \bar{\bx}\| \leq r_{\bx}$ and any $\bxi \in \partial \phi(\bx) \cap \partial g(\bx)$, let us define $\bz = \bx + \mu \bxi$. Then it holds that
% \begin{align*}
% F_{\mu}(\bar{\bz}) = F(\bar{\bx}) \leq F(\bx) = F_{\mu}(\bz),
% \end{align*}
% % where the equalities follow from \Cref{Prop: correspondence of stationary point and global minimizer} and the inequality from the local minimality of $\bar{\bx}$.
% which follow from \Cref{Prop: smoothness of DME} (iii) and the properties of stationary points established in \Cref{Prop: correspondence of stationary point and global minimizer} since $\bar{\bx}$, as a local minimizer of $F$, necessarily satisfies the stationarity condition for $F$. 
For any $\bx$ with $\|\bx - \bar{\bx}\| \le r_{\bx}$ and any 
$\bxi \in \partial \phi(\bx) \cap \partial g(\bx)$, define $\bz = \bx + \mu \bxi$.
Then, one has
\begin{align*}
  F_{\mu}(\bar{\bz}) = F(\bar{\bx}) \leq F(\bx) = F_{\mu}(\bz),
\end{align*}
where the equalities follow from Proposition~\ref{Prop: correspondence of stationary point and global minimizer}
and the inequality follows from the local minimality of $\bar{\bx}$. To determine $r_{\bz}$, we bound the distance:
\begin{align*}
\|\bz - \bar{\bz}\| &= \|\bx + \mu \bxi - (\bar{\bx} + \mu \bar{\bxi})\| \leq \|\bx - \bar{\bx}\| + \mu \|\bxi - \bar{\bxi}\|.
\end{align*}

We consider the two cases separately:
\begin{itemize}
  \item[(i)] If $g$ is $L_g$-smooth, then $\|\bxi - \bar{\bxi}\| \le L_g \|\bx - \bar{\bx}\|$, yielding
  \[
    \|\bz - \bar{\bz}\| \le (1 + \mu L_g)\|\bx - \bar{\bx}\| \le (1 + \mu L_g) r_{\bx}.
  \] 
  Taking $r_{\bz} = (1 + \mu L_g) r_{\bx}$ ensures that $\|\bz - \bar{\bz}\| \le r_{\bz}$.

  \item[(ii)] If $\sup_{\xi_g \in \partial g} \|\xi_g\| \le M_{\partial g}$, then
  $\|\bxi - \bar{\bxi}\| \le 2M_{\partial g}$, yielding
  \[
    \|\bz - \bar{\bz}\| \le \|\bx - \bar{\bx}\| + 2\mu M_{\partial g}
      \le r_{\bx} + 2\mu M_{\partial g}.
  \]
Thus, by setting $r_{\bz} := r_{\bx} + 2\mu M_{\partial g}$, we obtain $\|\bz - \bar{\bz}\| \le r_{\bz}$.
\end{itemize}
In both cases, $\bar{\bz}$ is a local minimizer of $F_{\mu}$ with radius $r_{\bz}$ as in \eqref{Eq: the relationship of rx and rz}.

Conversely, if \(\bar{\bz}\) is a local minimizer of \(F_{\mu}\) with radius \(r_{\bz}\), then for any \(\bz\) satisfying \(\| \bz - \bar{\bz} \| \leq r_{\bz} \), we have
\begin{align*}
    F(\textrm{prox}_{\mu \phi}(\bar{\bz})) &= F_{\mu}(\bar{\bz})  \leq F_{\mu}(\bz) \leq F(\textrm{prox}_{\mu g}(\bz))\\
    \textrm{prox}_{\mu \phi}(\bar{\bz}) &= \textrm{prox}_{\mu g}(\bar{\bz}).
\end{align*}
Similarly, it is evident to verify that for the radius \(r_{\bx}\) satisfying \eqref{Eq: the relationship of rx and rz}, it holds that
\begin{align}
% \label{Eq: the definitin of the local minimizer of F}
F(\textrm{prox}_{\mu \phi}(\bar{\bz})) \leq F(\bx)\text{, for any \(\bx\) satisfying \(\| \bx - \textrm{prox}_{\mu \phi}(\bz)\| \leq r_{\bx}\), } \notag
\end{align}
This implies that \(\textrm{prox}_{\mu \phi}(\bar{\bz})\) is a local minimizer of \(F\) and completes the proof.
\end{proof}
\subsection{Proof of \Cref{Prop: approximate correspondence}}
\label{App: proof of prop2.2}
For the complexity analysis, we rely on the correspondence between $\varepsilon$-stationary points established in \Cref{Prop: approximate correspondence}. We provide its proof below.
\begin{proof}
We first show that an $\varepsilon$-stationary point of $F_{\mu}$ 
induces an $\varepsilon$-critical point of $F$.
Let $\bar{\bz}$ be a point satisfying $\|\nabla F_{\mu}(\bar{\bz})\|\le\varepsilon$ and set
\[
  \bar{\bx} := \mathrm{prox}_{\mu \phi}(\bar{\bz}), \qquad
  \bar{\by} := \mathrm{prox}_{\mu g}(\bar{\bz}).
\]
Using \eqref{Eq: the gradient of Moreau envelope}, we have
\[
  \bar{\bxi}_{\phi} := \mu^{-1}(\bar{\bz}-\bar{\bx}) \in \partial \phi(\bar{\bx}),
  \qquad
  \bar{\bxi}_{g} := \mu^{-1}(\bar{\bz}-\bar{\by}) \in \partial g(\bar{\by}).
\]
Combining these with \eqref{Eq: the gradient of Moreau envelope} yields
\[
  \bar{\bxi}_{\phi} - \bar{\bxi}_{g}
    = \mu^{-1}(\bar{\by}-\bar{\bx})
    = \nabla F_{\mu}(\bar{\bz}).
\]
It follows that
\begin{align*}
  \max\bigl\{\|\bar{\bxi}_{\phi}-\bar{\bxi}_{g}\|,
             \|\bar{\bx}-\bar{\by}\|\bigr\}  = \max\bigl\{\|\nabla F_{\mu}(\bar{\bz})\|,
                  \mu\|\nabla F_{\mu}(\bar{\bz})\|\bigr\} = \max\{1,\mu\}\,\|\nabla F_{\mu}(\bar{\bz})\| \leq \varepsilon.
\end{align*}
This implies that $\bar{\bx}$ is an $\varepsilon$-critical point of $F$ in the sense of Definition~\ref{Def: epsilon-critical point in DC}.

Conversely, suppose that $\bar{\bx}$ is an $\varepsilon$-critical point of $F$, so that there exist $\bar{\by}\in\RR^n$ and
$\bar{\bxi}_{\phi}\in\partial\phi(\bar{\bx})$,
$\bar{\bxi}_{g}\in\partial g(\bar{\by})$ satisfying
\[
  \max\bigl\{\|\bar{\bxi}_{\phi}-\bar{\bxi}_{g}\|,
             \|\bar{\bx}-\bar{\by}\|\bigr\} \le \varepsilon.
\]
By defining
\[
  \bar{\bz} := \bar{\bx} + \mu \bar{\bxi}_{\phi}
            =  \bar{\by} + \mu \bar{\bxi}_{g},
\] and using the preimage characterization of the proximal operator, we obtain
\[
  \mathrm{prox}_{\mu \phi}(\bar{\bz}) = \bar{\bx},
  \qquad
  \mathrm{prox}_{\mu g}(\bar{\bz}) = \bar{\by},
\]
which implies
\begin{align*} 
  \|\nabla F_{\mu}(\bar{\bz})\|
    &= \mu^{-1}\bigl\|\mathrm{prox}_{\mu g}(\bar{\bz}) 
                     - \mathrm{prox}_{\mu \phi}(\bar{\bz})\bigr\|  \\
    &= \mu^{-1}\|\bar{\by}-\bar{\bx}\|
     \leq \varepsilon.
\end{align*}
Hence $\bar{\bz}$ is an $\varepsilon$-stationary point of $F_{\mu}$, which completes the proof.
\end{proof}
